# Supplementary material for: Borrowing Human Senses: Comment-Aware Self-Training for Social Media Multimodal Classification
Source: arXiv:2303.15016 source file (2023-03-27)
Supplement: Supplementary file 1 [file case_appendix.tex]

\begin{figure}[ht]
\centering
\includegraphics[width=0.9\columnwidth]{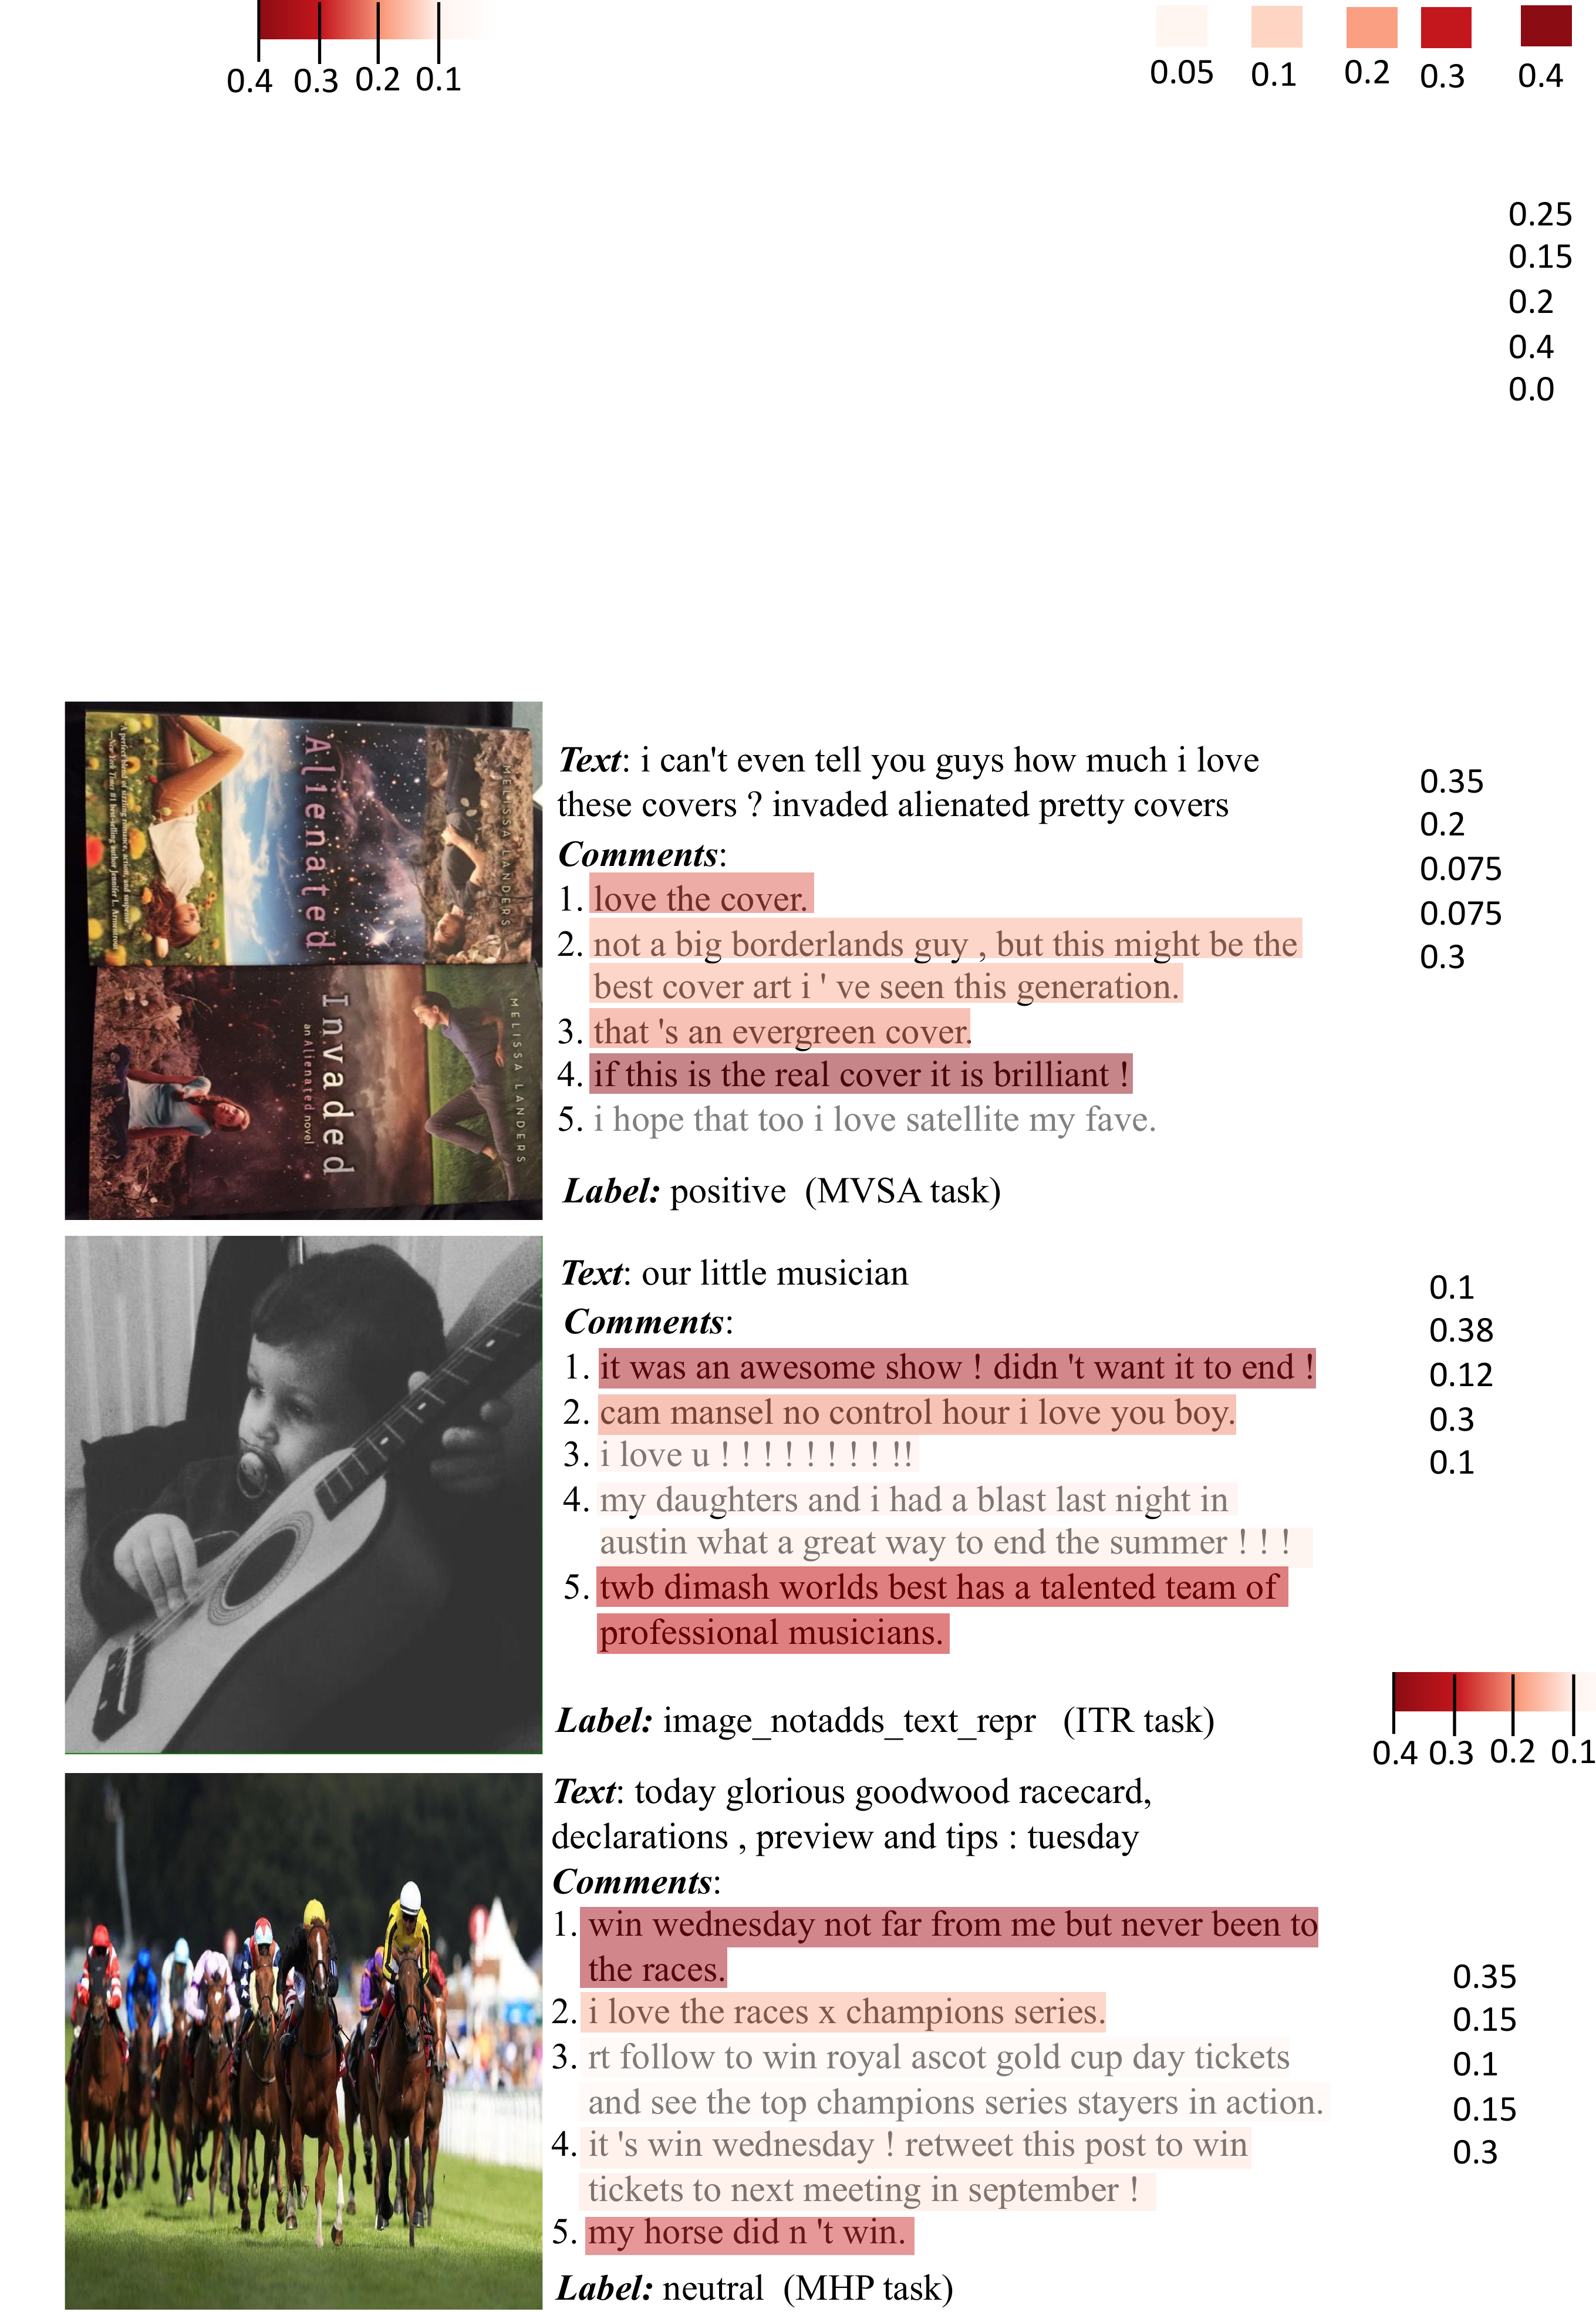}
% \caption{Visualization of attention heatmaps over the retrieved comments. From up to down shows the sampled visualized attention cases from MVSA, ITR, and MHP benchmark. Deeper colors indicate higher attention weights. 
% }
\caption{From up to down shows the sampled visualized attention cases from MVSA, ITR, and MHP benchmark. 
}

\label{fig:case_study}
\end{figure}
